# Supplementary material for: Towards Complex Dynamic Physics System Simulation with Graph Neural ODEs
Source: arXiv:2305.12334 source file (2023-06-30)
Supplement: Supplementary file 1 [file 9_appendix.tex]

\begin{figure*}[t]
\centering
\subfigure{
\includegraphics[width=.20\linewidth]{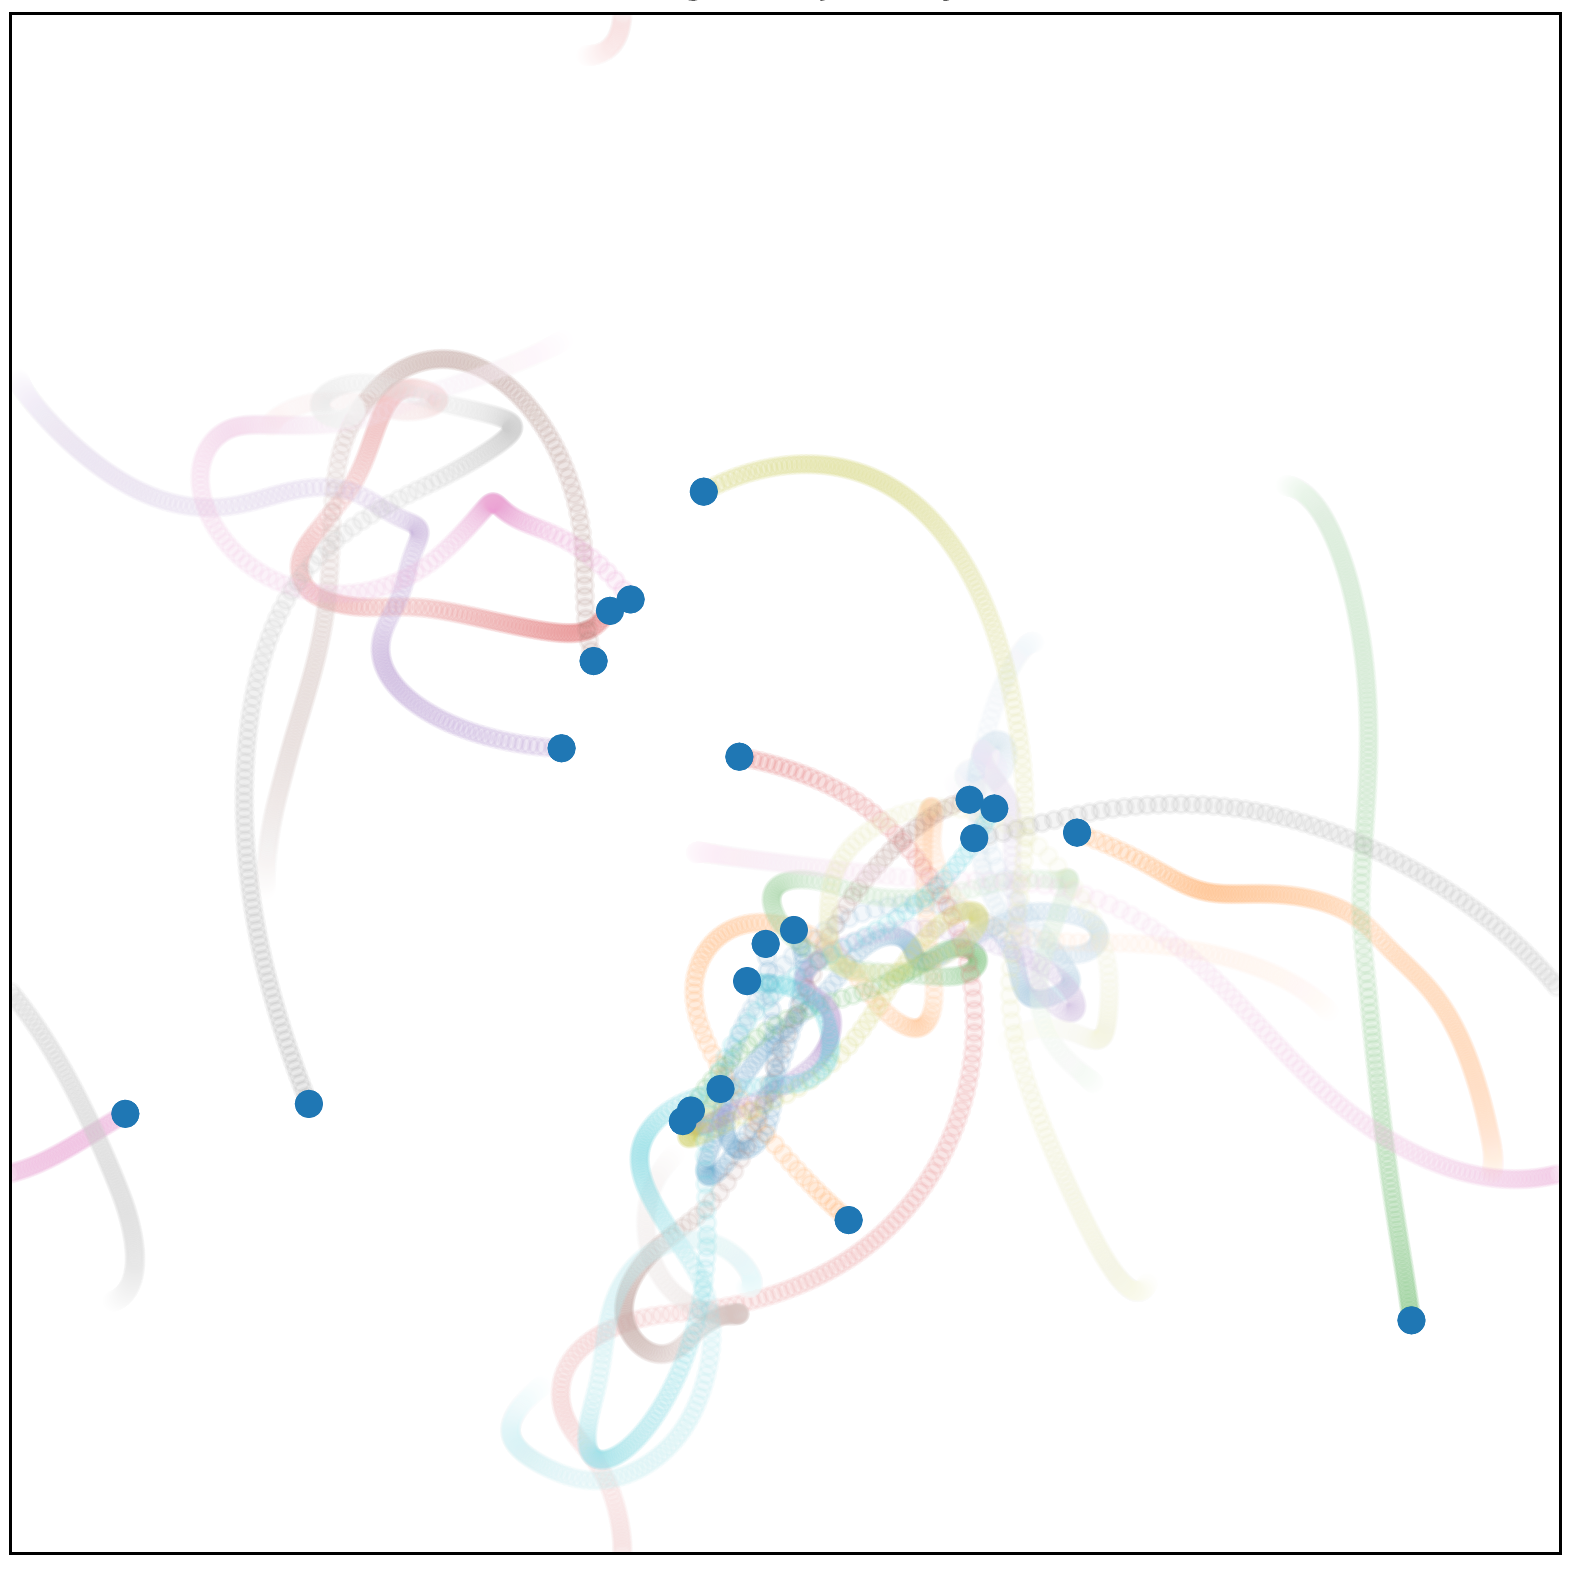}
\label{apx:target_c}
}
\subfigure{
\includegraphics[width=.20\linewidth]{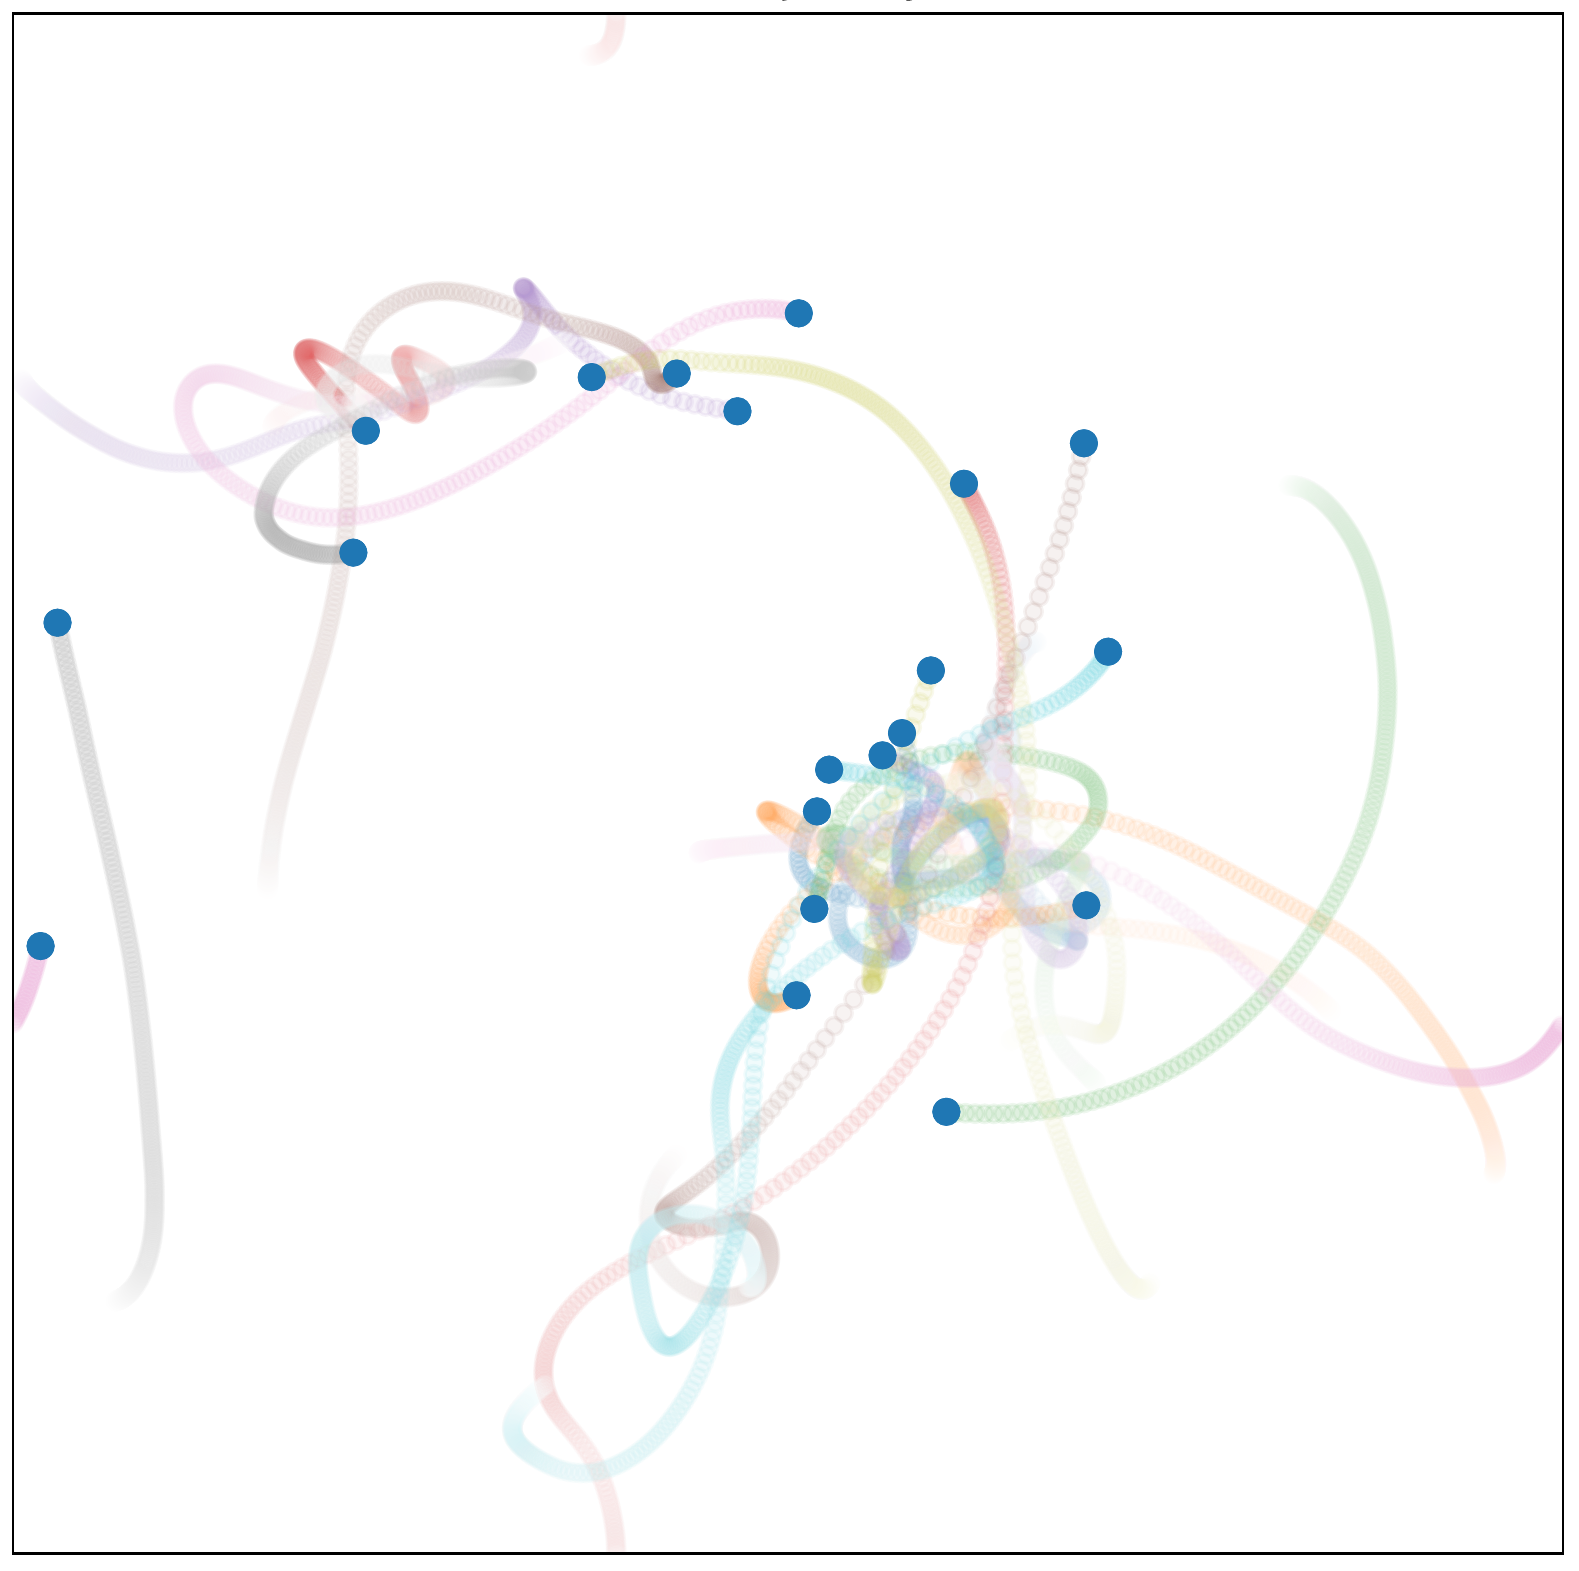}
\label{apx:GN_c}
}
\subfigure{
\includegraphics[width=.20\linewidth]{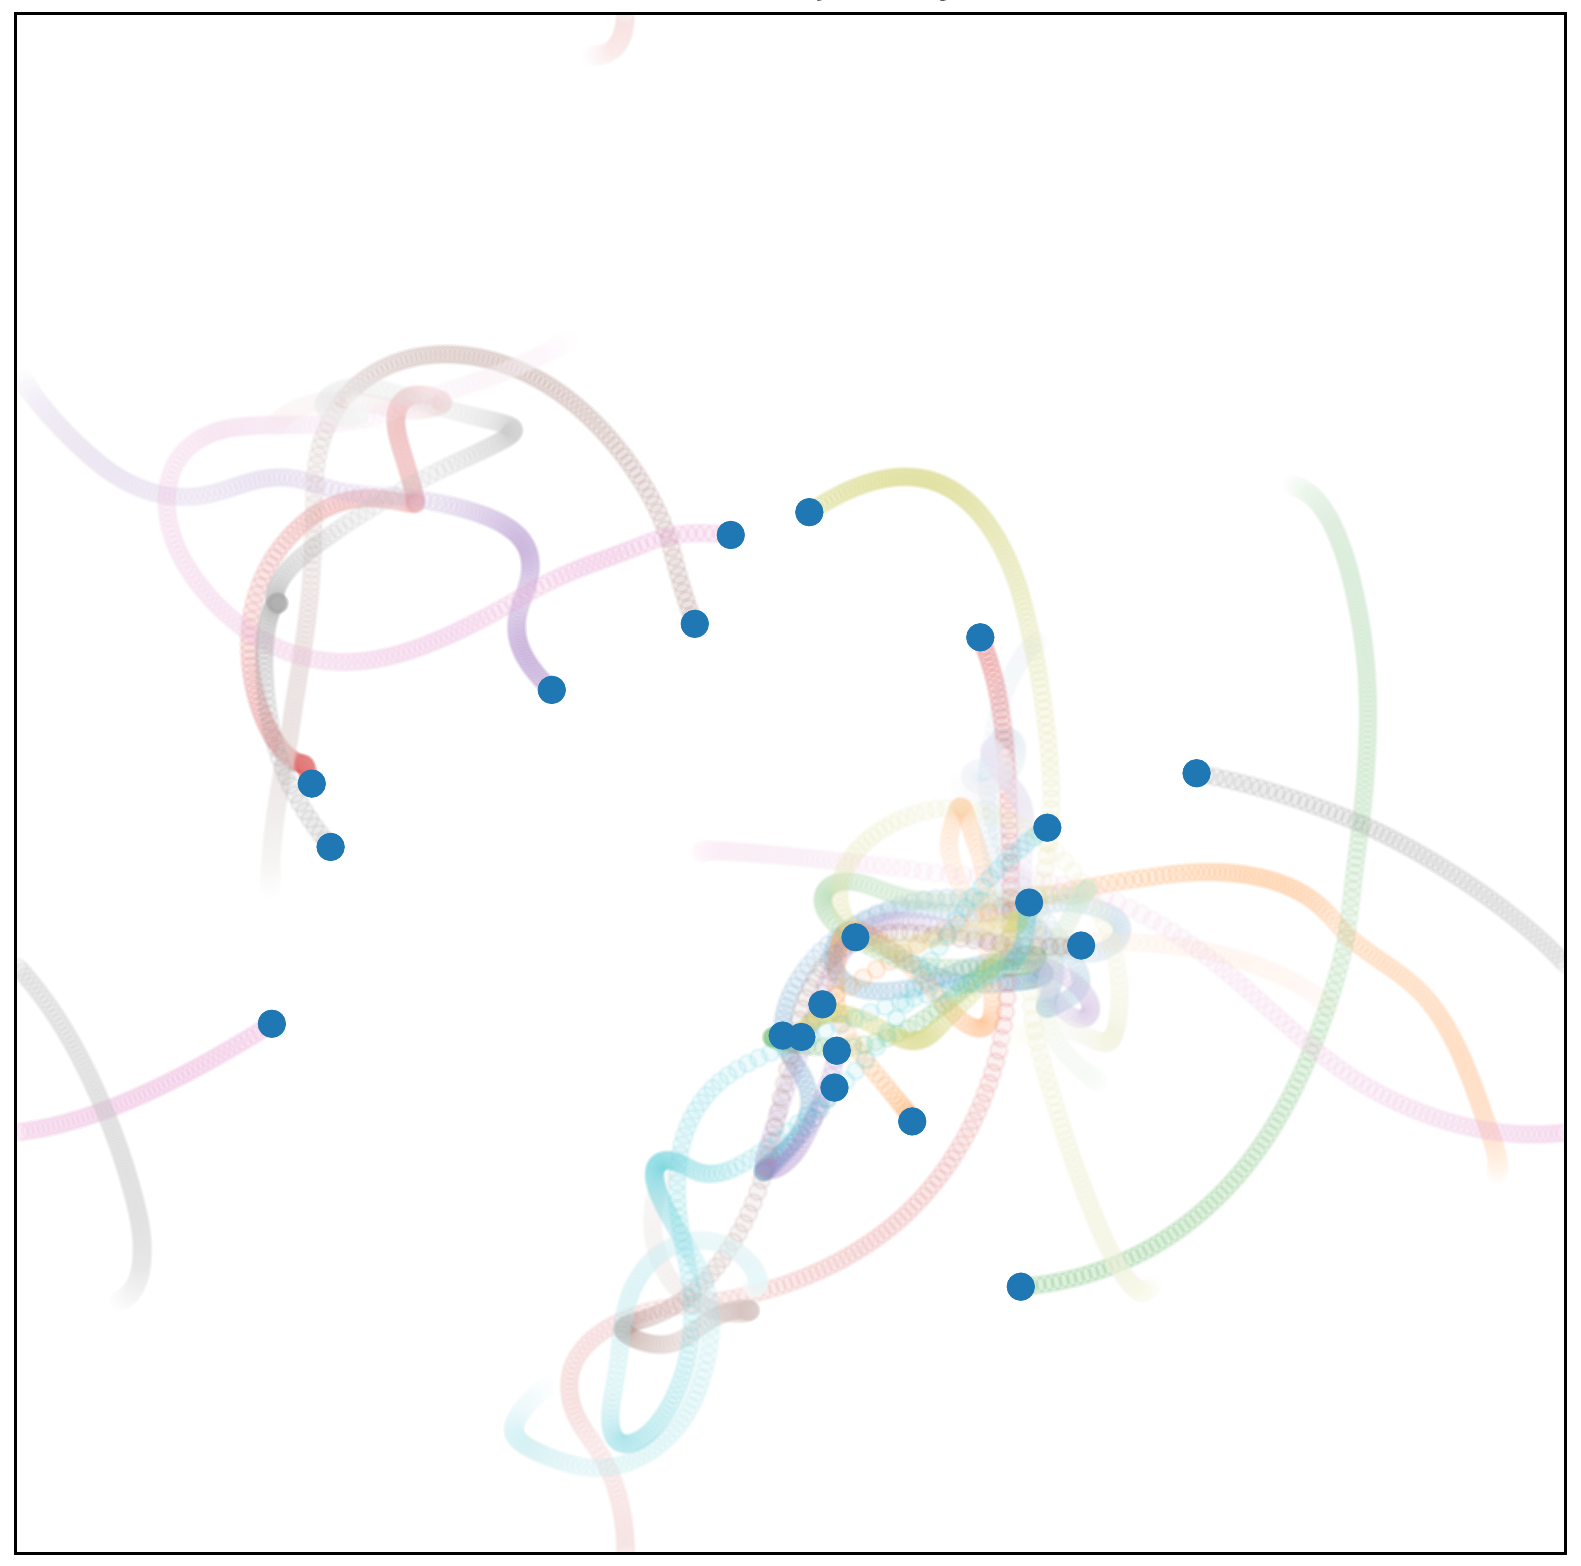}
\label{apx:HDGN_c}
}
\subfigure{
\includegraphics[width=.20\linewidth]{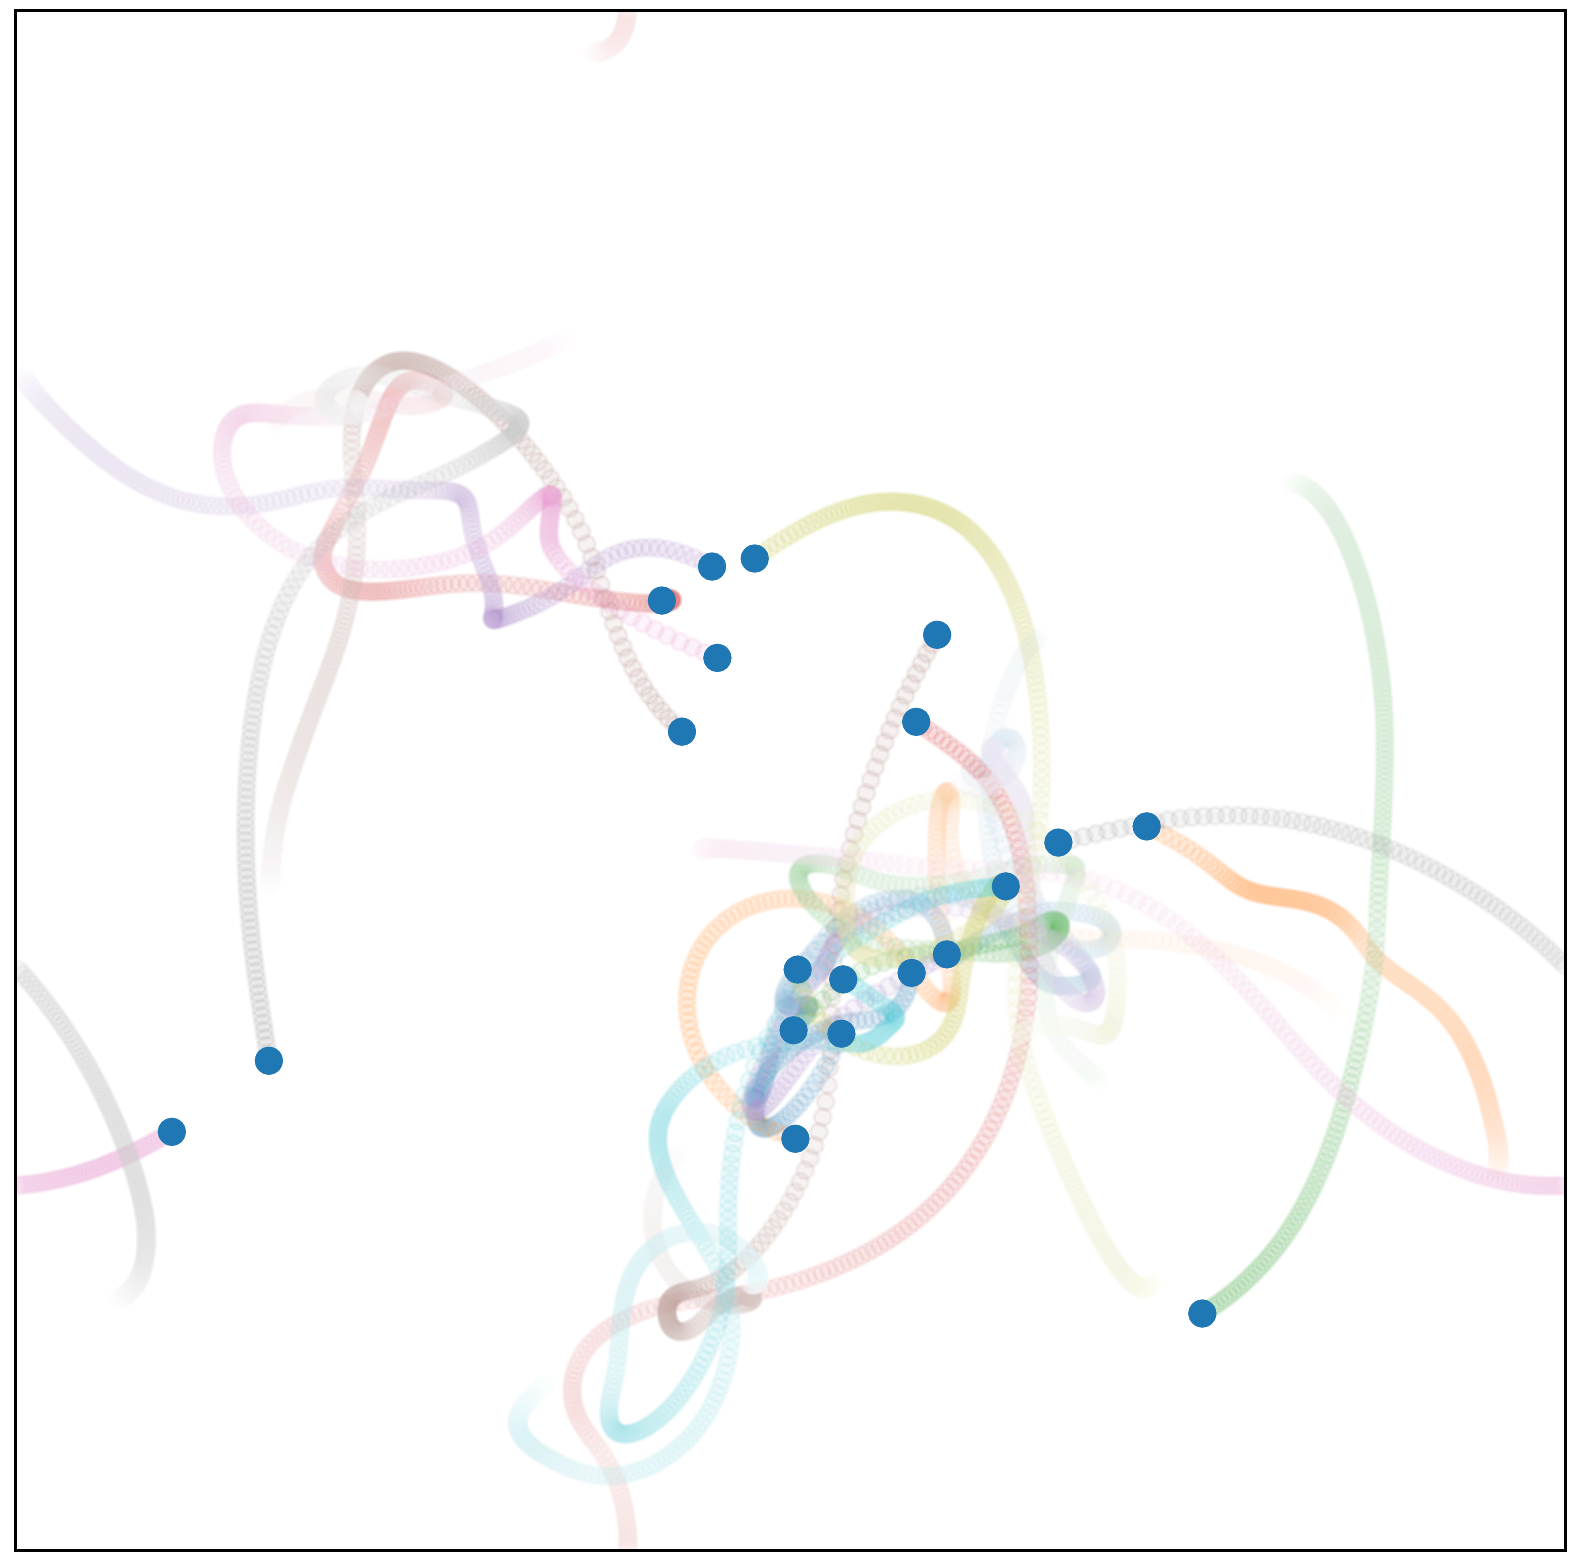}
\label{apx:GNSTODE_c}
}
\caption{
Rollout of different methods for coulomb dataset with scale 20, density 0.42, target step 1,.
}
\label{fig:appendix_c}
\end{figure*}

\begin{figure*}[t]
\centering
\subfigure{
\includegraphics[width=.20\linewidth]{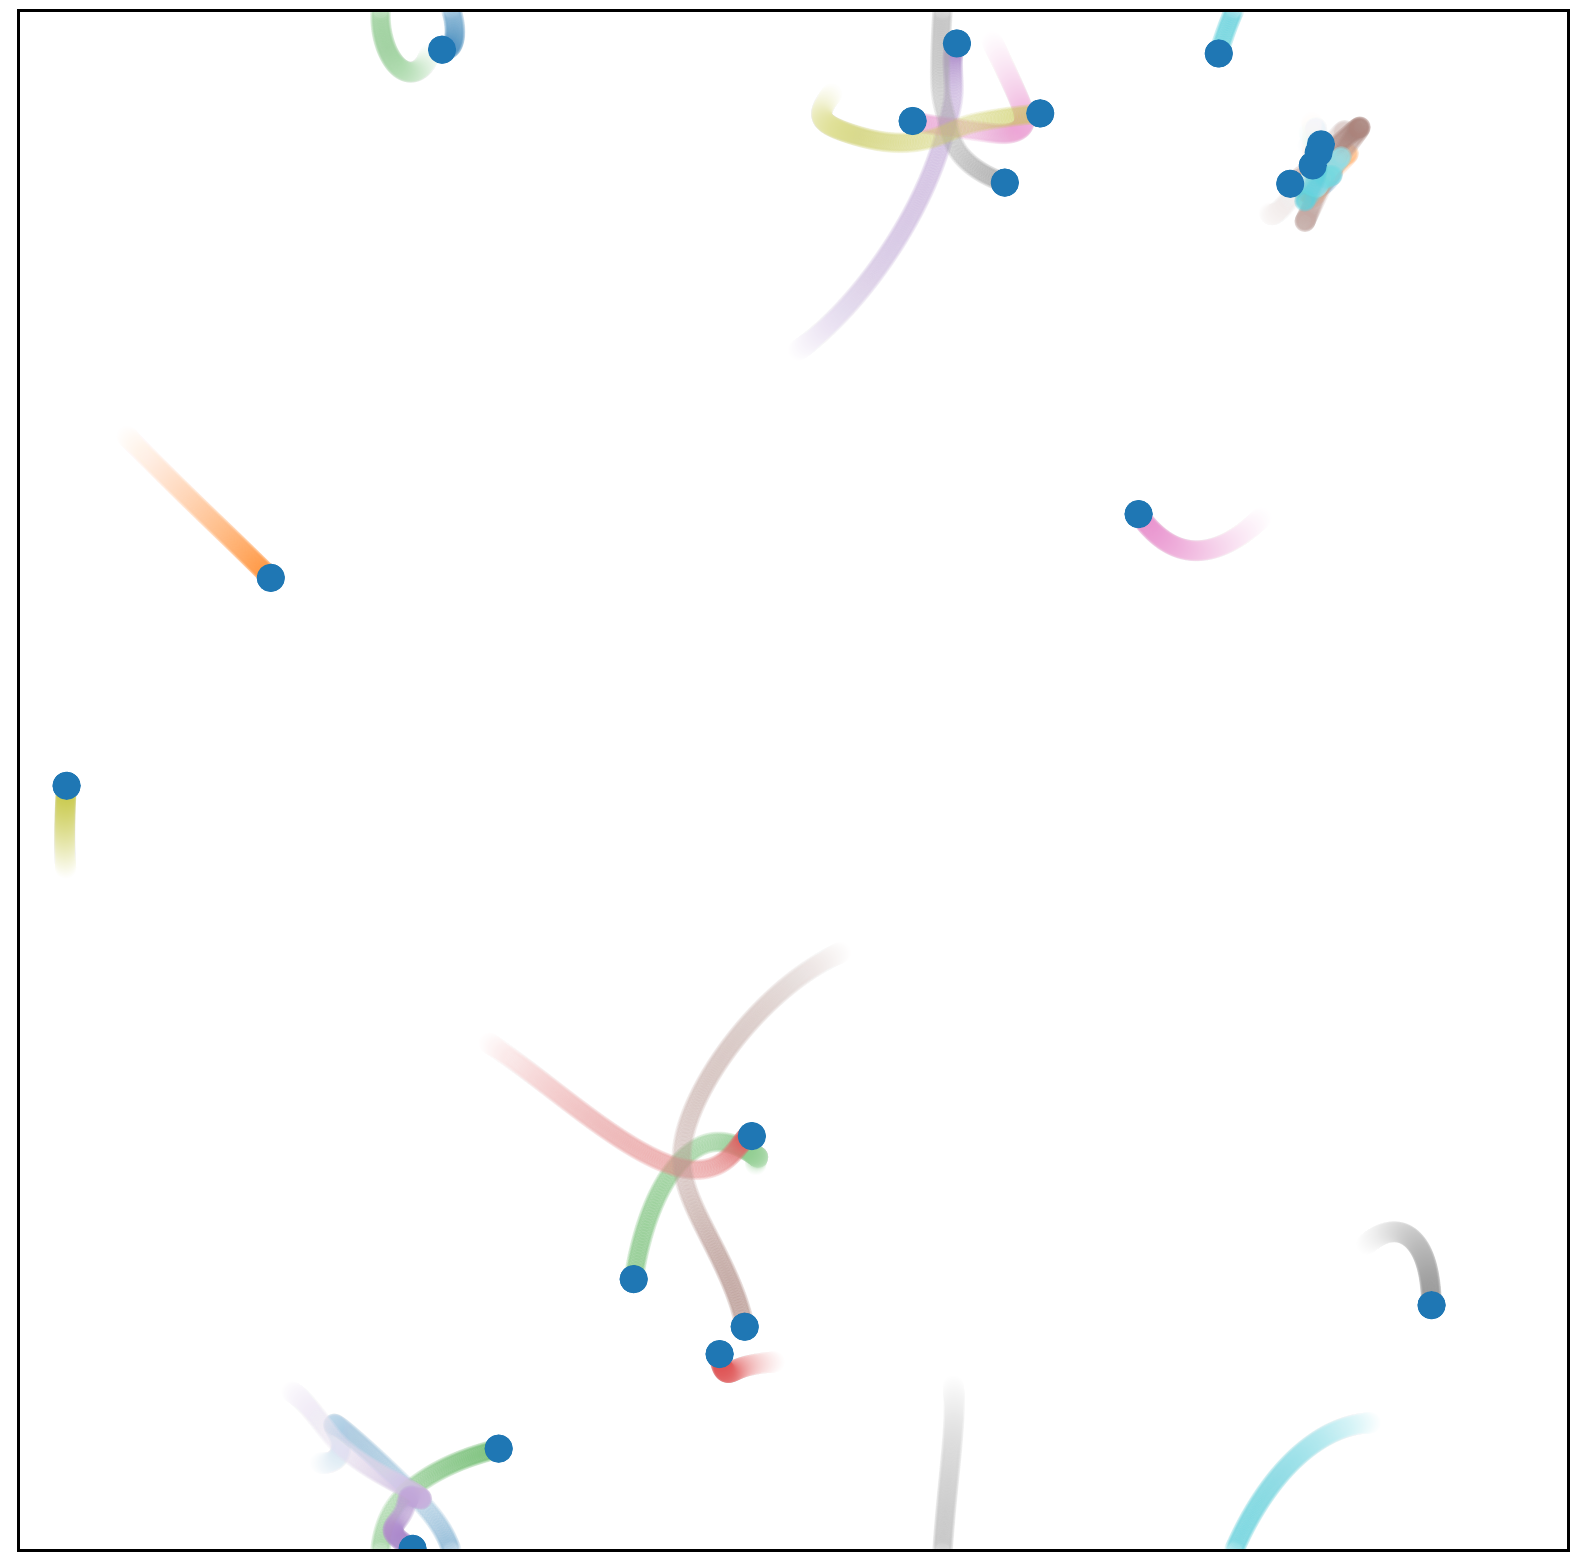}
\label{apx:target_15.5}
}
\subfigure{
\includegraphics[width=.20\linewidth]{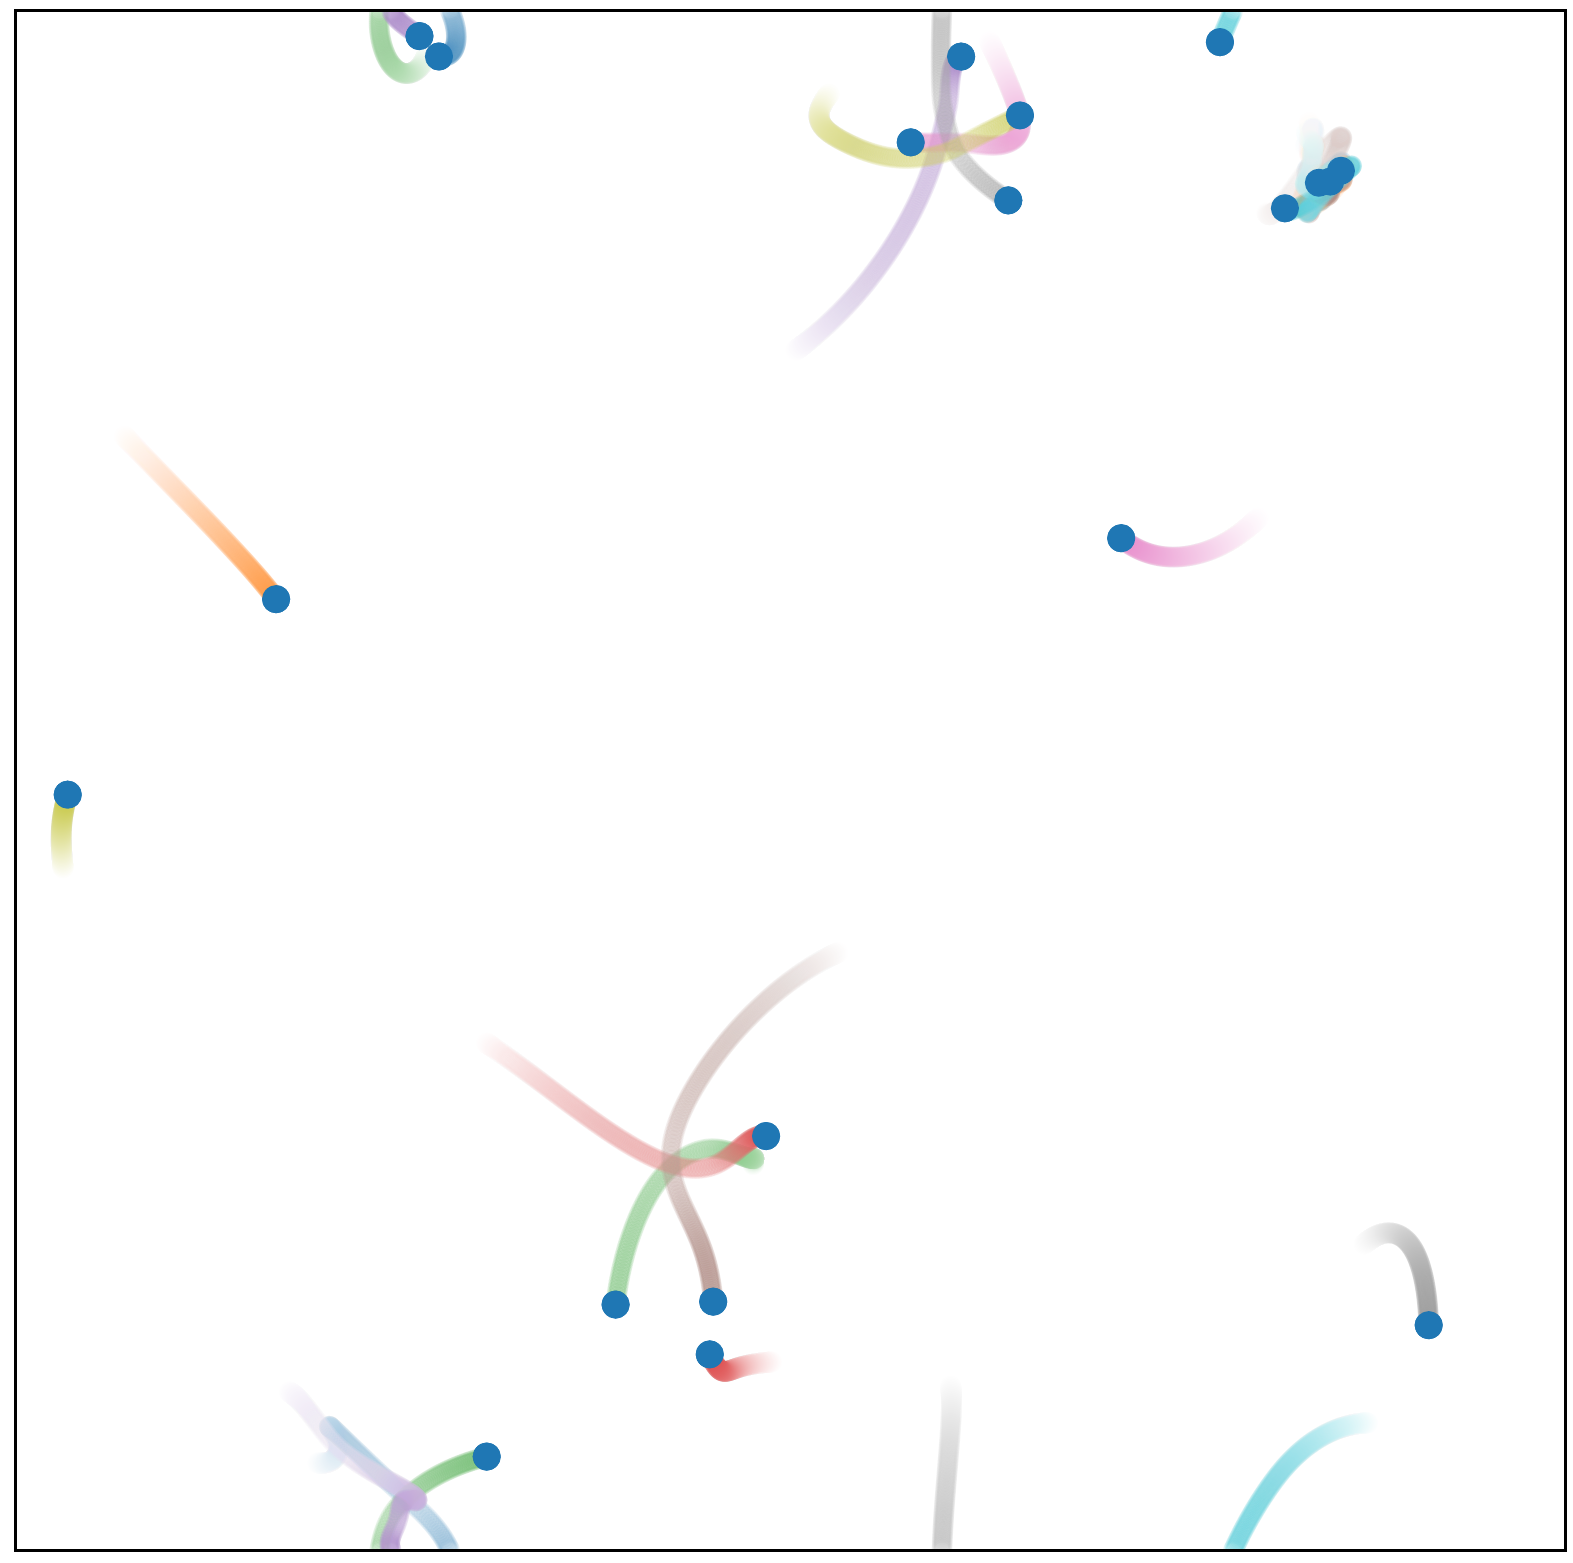}
\label{apx:GN_15.5}
}
\subfigure{
\includegraphics[width=.20\linewidth]{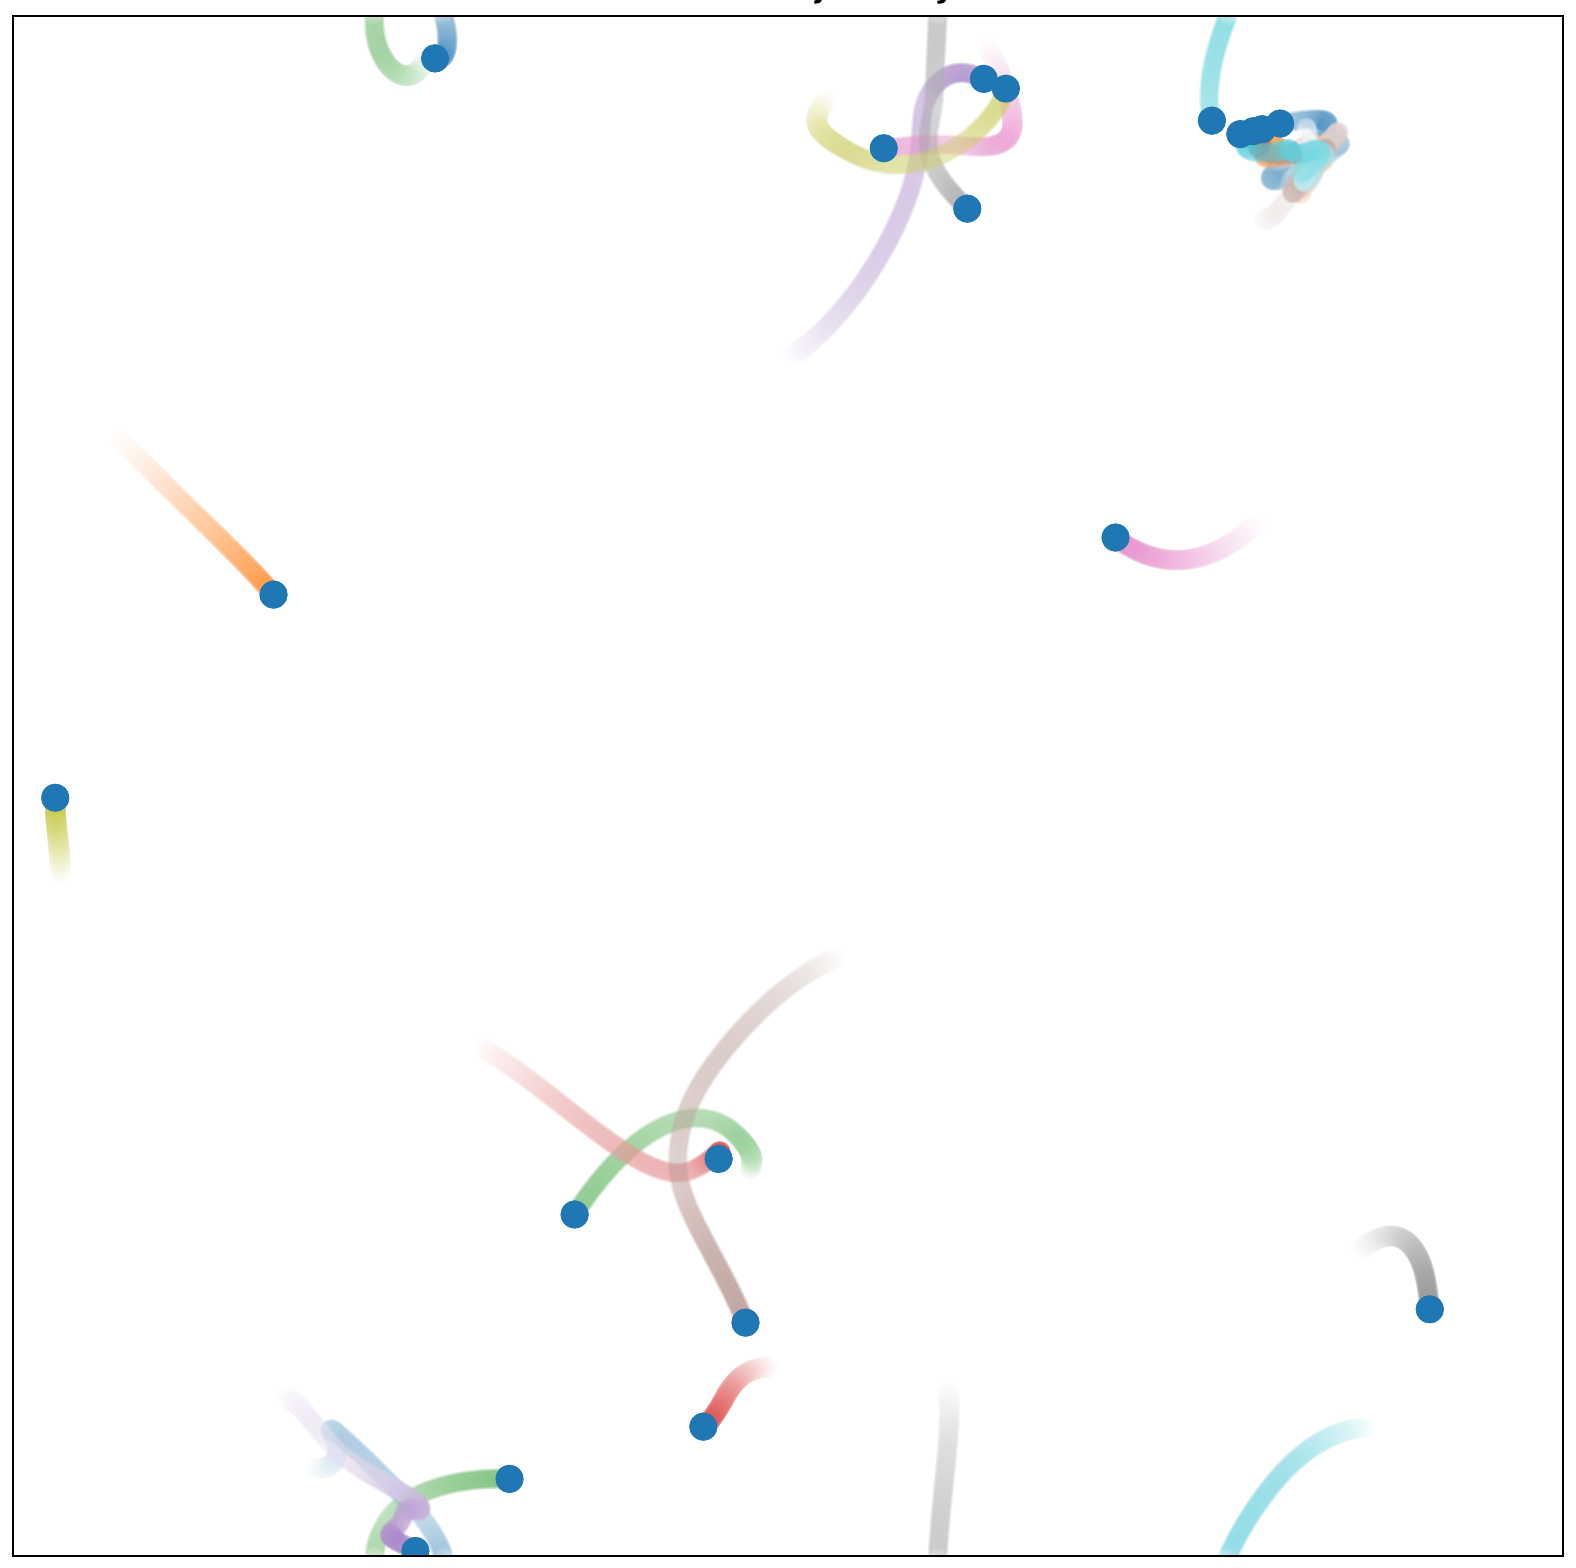}
\label{apx:HDGN_15.5}
}
\subfigure{
\includegraphics[width=.20\linewidth]{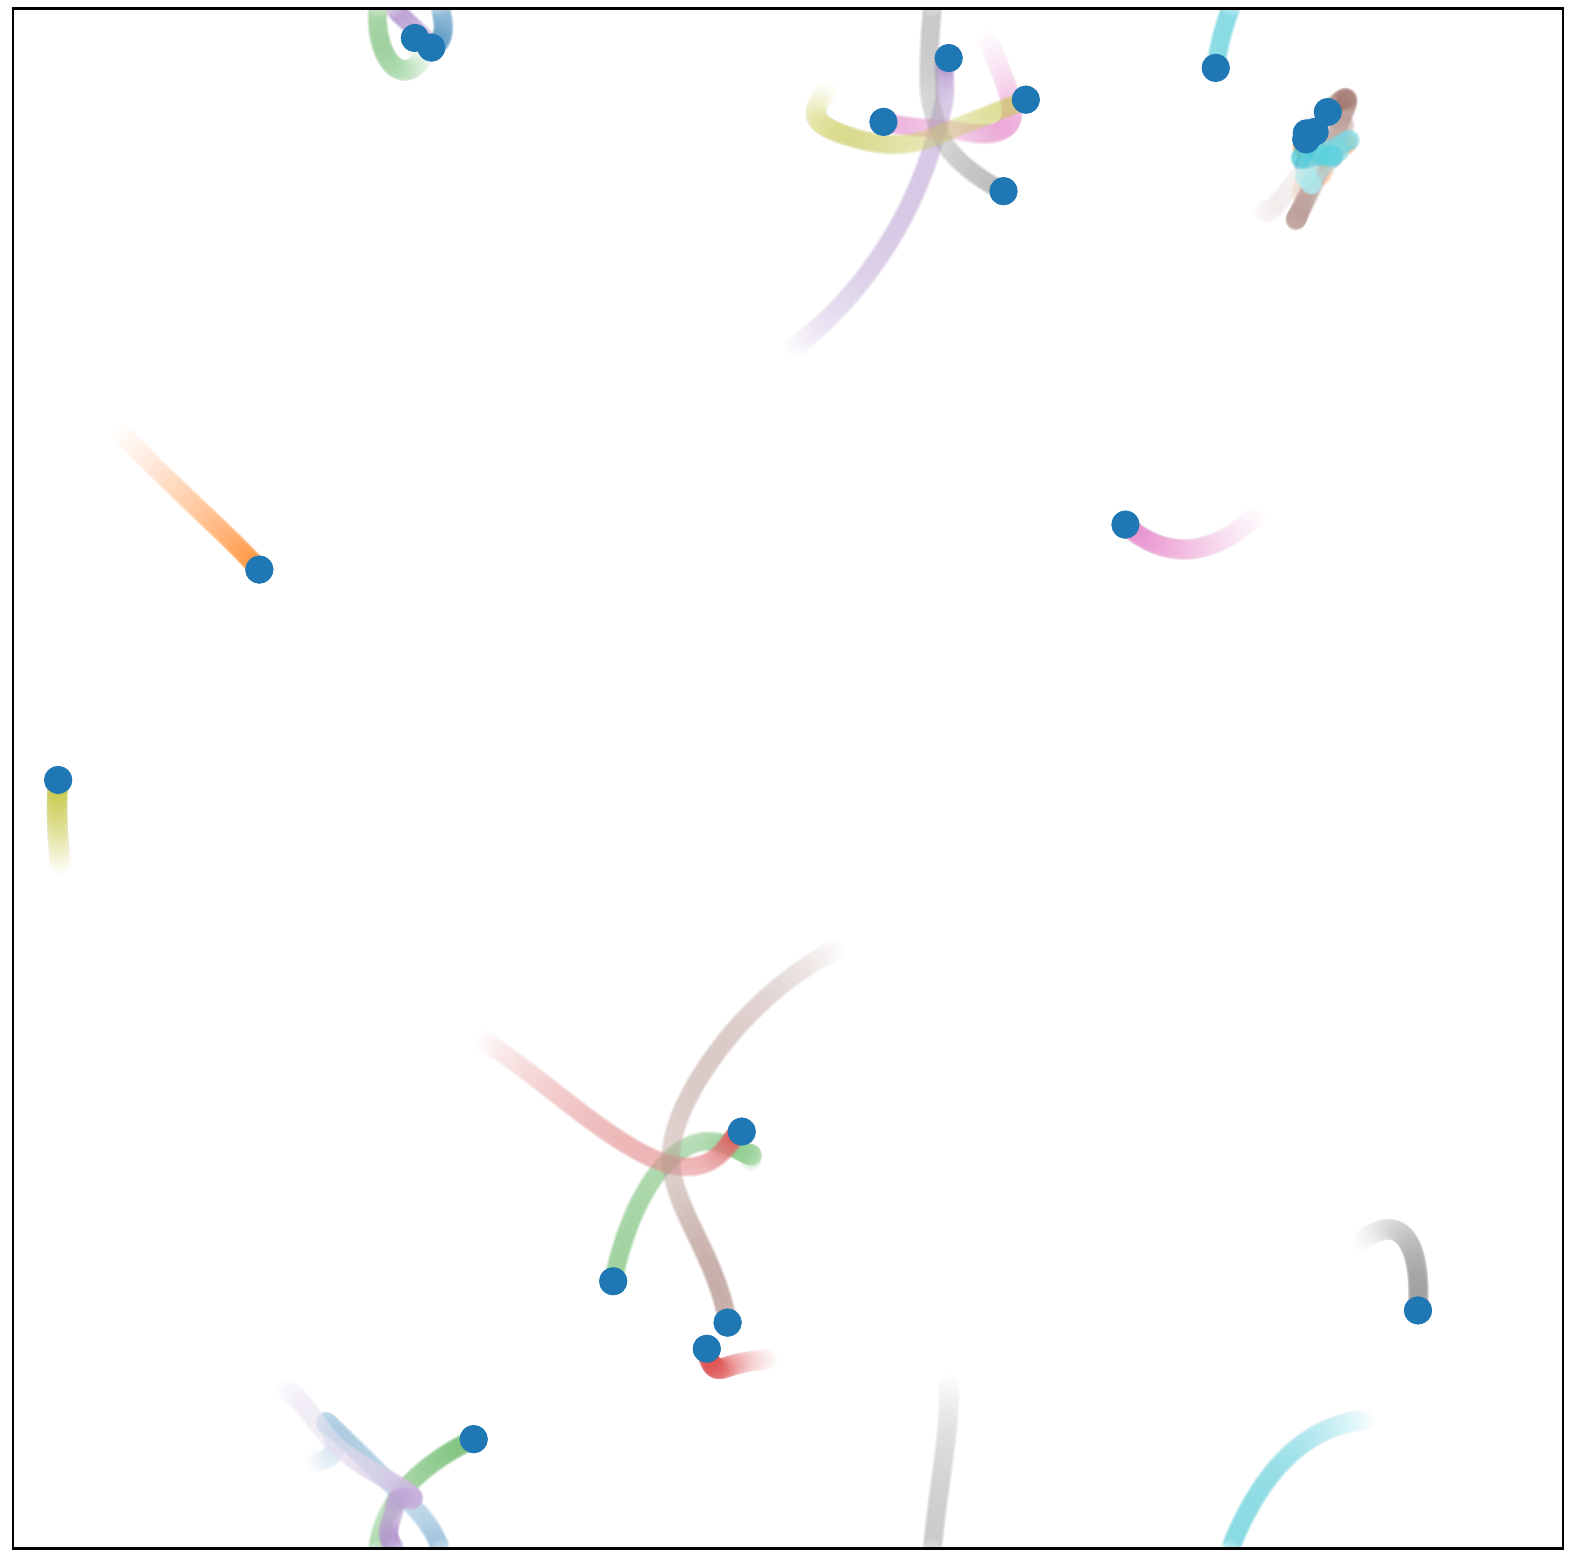}
\label{apx:GNSTODE_15.5}
}
\caption{
Rollout of different methods for gravity dataset with scale 20, density 1.63, target step 1,.
}
\label{fig:appendix_15.5}
\end{figure*}

we draw the trajectory different datasets for visualization, first picture is the target, and we compare GN, HDGN and our method \method
